# Supplementary material for: FDSOI Process Based MIV-transistor Utilization for Standard Cell Designs in Monolithic 3D Integration
Source: arXiv:2306.14032 source file (2023-06-24)
Supplement: Supplementary file 1 [file Section_appendix.tex]

\clearpage

\appendix
\begin{table}[h]
    \centering
    \label{tab:Param_ranges}
\caption{Level 70 Spice parameters used in extraction  \cite{hspice_mosfet_models}}
    \begin{tabular}{|c|p{6.5cm}|}
         \hline
        \textbf{Parameter} & \textbf{Description}  \\
        \hline 
        CDSC & Drain/Source to channel coupling capacitance  \\
        \hline
        CDSCD & Drain-bias sensitivity of CDSC  \\
        \hline
        U0 & Mobility at Temp = Tnom  \\
        \hline
        UA & First-order mobility degradation coefficient  \\
        \hline
        UB & Second-order mobility degradation coefficient  \\
        \hline
        UD & Coulomb scattering factor for mobility  \\
        \hline
        UCS & Mobility exponent factor in mobMod=4  \\ 
        \hline
        DVT0 & First coefficient of short-channel effect on Vth  \\ 
        \hline
        DVT1 & Second coefficient of short-channel effect on Vth  \\ 
        \hline
        PVAG & Gate dependence of Early voltage  \\ 
        \hline
        ETAB & Body-bias coefficient for the subthreshold DIBL effect  \\ 
        \hline
        VSAT & Saturation velocity at Temp=Tnom  \\ 
        \hline
        VTH0 & Threshold voltage @Vbs=0 for long and wide device  \\ 
        \hline
        CKAPPA & Coefficient for lightly doped region overlap capacitance fringing field capacitance  \\ 
        \hline
        
        CGDO & Non LDD region drain-gate overlap capacitance per channel length  \\ 
        \hline
        CGSO & Non LDD region source-gate overlap capacitance per channel length  \\ 
        \hline
        CGSL &Light doped source-gate region overlap capacitance  \\ 
        \hline
        CGDL & Light doped drain-gate region overlap capacitance  \\ 
        \hline
        CF & Gate to source/drain fringing field capacitance   \\ 
        \hline 
        MOIN & Coefficient for the gate-bias dependent surface potential \\
        \hline 
        DELVT & Threshold voltage adjust for C-V  \\ 
        \hline 
    \end{tabular}
\end{table}
